# Supplementary material for: Dynamic Explanation Emphasis in Human-XAI Interaction with Communication Robot
Source: arXiv:2403.14550 source file (2024-03-21)
Supplement: Supplementary file 1 [file 99_appendix.tex]

\section*{Appendix}
aaa
